# Supplementary material for: Feed-forward Uncertainty Propagation in Belief and Neural Networks
Source: arXiv:1803.10590 source file (2018-11-01)
Supplement: Supplementary file 1 [file old_appendix_exps.tex]

\paragraph{Input Variance in MLP}
%%
We checked the effect of varying the input noise variance in the MNIST-MLP model. The results shown in~\cref{fig:input_var} indicate that increased input variance leads to more robust models.
\begin{figure}[t]
\centering
\resizebox{\linewidth}{!}{
\includegraphics[width=0.5\linewidth]{fig/exps/MLP/var/stability_acc.pdf}%
\ \includegraphics[width=0.5\linewidth]{fig/exps/MLP/var/stability1_acc.pdf}%
}
\caption{Effect of increasing input variance in MNIST-MLP.\label{fig:input_var}}
\end{figure}
%%
%
%
%\subsection{Details of Learning LeNet-Bernoulli model}
%\begin{figure}[!t]
%\begin{tabular}{cc}%
%\begin{tabular}{c}%
%\includegraphics[width=0.5\linewidth]{fig/exps/LeNetB/view/t_loss.pdf}%
%\end{tabular}%
%\begin{tabular}{c}%
%s\includegraphics[width=0.5\linewidth]{fig/exps/LeNetB/view/v_acc.pdf}%
%\end{tabular}%
%\end{tabular}
%\caption{LeNet with Bernoulli hidden units. }
%\end{figure}
%
\paragraph{Learning Behavior in LeNet}
\cref{fig:Lenet-losses-B,fig:Lenet-losses-R} show learning plots corresponding to the networks compared in \cref{fig:LeNet}. Also our method performs better in training loss, the validation loss quickly saturates and the further learning progress is not useful and may be actually harmful. While the is no visible increase of validation accuracy due to overfitting, there is certainly some loss of stability if we select the model not with the best validation loss but just the last one.
Validation error of S-BN in~\cref{fig:Lenet-losses-R} is clearly better and its validation error is by a half of percent better. We don not know why this is so. There are several things entangled including the normalization based on batch statistics and the optimization algorithm. %whether this is some systematic property of BN, that shold be 
%%
\begin{figure}[t]
\resizebox{\linewidth}{!}{
\begin{tabular}{c}%
\includegraphics[width=0.5\linewidth]{fig/exps/LeNetB/view/t_loss.pdf}\,%
\end{tabular}%
\begin{tabular}{c}%
\includegraphics[width=0.5\linewidth]{fig/exps/LeNetB/view/v_acc.pdf}%
\end{tabular}%
}
\caption{Training progress of LeNet with Logistic Bernoulli activations. A significant difference between training loss and validation loss is observed.
%In this case we observe severe overfitting. The stability to Gaussian noise is improved compared to standard counterparts and for {\tt V-Norm} variant it can be pushed furthesr by increasing the assumed input variance. But improvement of stability to adversarial attacks is not observed
\label{fig:Lenet-losses-B}}
\end{figure}
%
\begin{figure}[!t]
\resizebox{\linewidth}{!}{
\begin{tabular}{c}%
\includegraphics[width=0.5\linewidth]{fig/exps/LeNet/view/t_loss.pdf}\,%
\end{tabular}%
\begin{tabular}{c}%
\includegraphics[width=0.5\linewidth]{fig/exps/LeNet/view/v_acc.pdf}%
\end{tabular}%
}
\caption{Training progress of LeNet with ReLU activations. The training loss quickly goes below $10^{-5}$ while validation losses stay well above $10^{-2}$ (dotted lines), which indicates big overfitting. BN appears to suffer less from overfitting and achieves higher accuracy, for which we do not have a good explanation.
%In this case we observe severe overfitting. The stability to Gaussian noise is improved compared to standard counterparts and for {\tt V-Norm} variant it can be pushed furthesr by increasing the assumed input variance. But improvement of stability to adversarial attacks is not observed.
\label{fig:Lenet-losses-R}}
\end{figure}
%
\paragraph{Input and Activation Variance in LeNet}\label{sec:input_var}
We studied the effect of varying input variance in LeNet-ReLU, shown in~\cref{fig:LeNet-ReLU-ivar}. While there is some slight improvement in stability to Gaussian noise, in stability to adversarial noise we don't see such dependency and varNN model does not improve over the baseline stdNN. Similar picture holds when we mare ReLU a stochastic rectifier~\cite{Bengio2013EstimatingOP}, adding the noise to the signal in front of ReLU. As everywhere in our framework, we do not sample this noise, but just use its variance. \cref{fig:LeNet-ReLU-avar} shows there was no noticeable effect when increasing this variance. This indicates that the model has many degrees of freedom to fit to the data so that increasing the variances does not induce a significant regularization.
%
%
\begin{figure}[!t]
{\centering
\resizebox{\linewidth}{!}{
\includegraphics[width=0.5\linewidth]{fig/exps/LeNet/var1/stability_acc.pdf}%
\ \includegraphics[width=0.5\linewidth]{fig/exps/LeNet/var1/stability1_acc.pdf}%
}\\}
\caption{Effect of increasing input variance in LeNet-ReLU. While it can improve stability to Gaussian noise, in stability to adversarial attacks the effect is hardly observed and there is no improvement over the standard network. We believe this is due to the severe overfitting.
\label{fig:LeNet-ReLU-ivar}}
\end{figure}
%%
\begin{figure}[!t]
{\centering
\resizebox{\linewidth}{!}{
\includegraphics[width=0.5\linewidth]{fig/exps/LeNet/avar/stability_acc.pdf}%
\ \includegraphics[width=0.5\linewidth]{fig/exps/LeNet/avar/stability1_acc.pdf}%
}\\}
\caption{Increasing injected noise in front of activations in LeNet-ReLU: small improvement to Gaussian noise but no effect observed in adversarial perturbations. We believe this is due to the severe overfitting.\label{fig:LeNet-ReLU-avar}}
\end{figure}
%
